# Supplementary material for: Requirements for a processing-node quantum repeater on a real-world fiber grid
Source: arXiv:2207.10579 source file (2023-10-20)
Supplement: Supplementary file 1 [file abstract_model_appendix.tex]

\section{Abstract model}
\label{appendix:sec_abstract_model}
