# Supplementary material for: Requirements for a processing-node quantum repeater on a real-world fiber grid
Source: arXiv:2207.10579 source file (2023-10-20)
Supplement: Supplementary file 2 [file remote_teleportation_appendix.tex]

\section{Remote state preparation and quantum teleportation}
\label{sec:appendix_rsp_teleportation}
